# Supplementary material for: A Complete Active Space Self-Consistent Field approach for molecules in QED environments
Source: arXiv:2503.16417 source file (2025-06-10)
Supplement: Supplementary file 1 [file SI_QED_CASSCF.pdf]

**Supporting Information:**

**A Complete Active Space Self-Consistent Field  
approach for molecules in QED environments**

Riccardo Alessandro,<sup>†</sup> Henrik Koch,<sup>‡</sup> and Enrico Ronca<sup>\*,†</sup>

*<sup>†</sup>Dipartimento di Chimica, Biologia e Biotecnologie, Università degli Studi di Perugia, Via  
Elce di Sotto, 8, 06123, Perugia, Italy*

*<sup>‡</sup>Department of Chemistry, Norwegian University of Science and Technology, 7491  
Trondheim, Norway*

E-mail: [enrico.ronca@unipg.it](mailto:enrico.ronca@unipg.it)

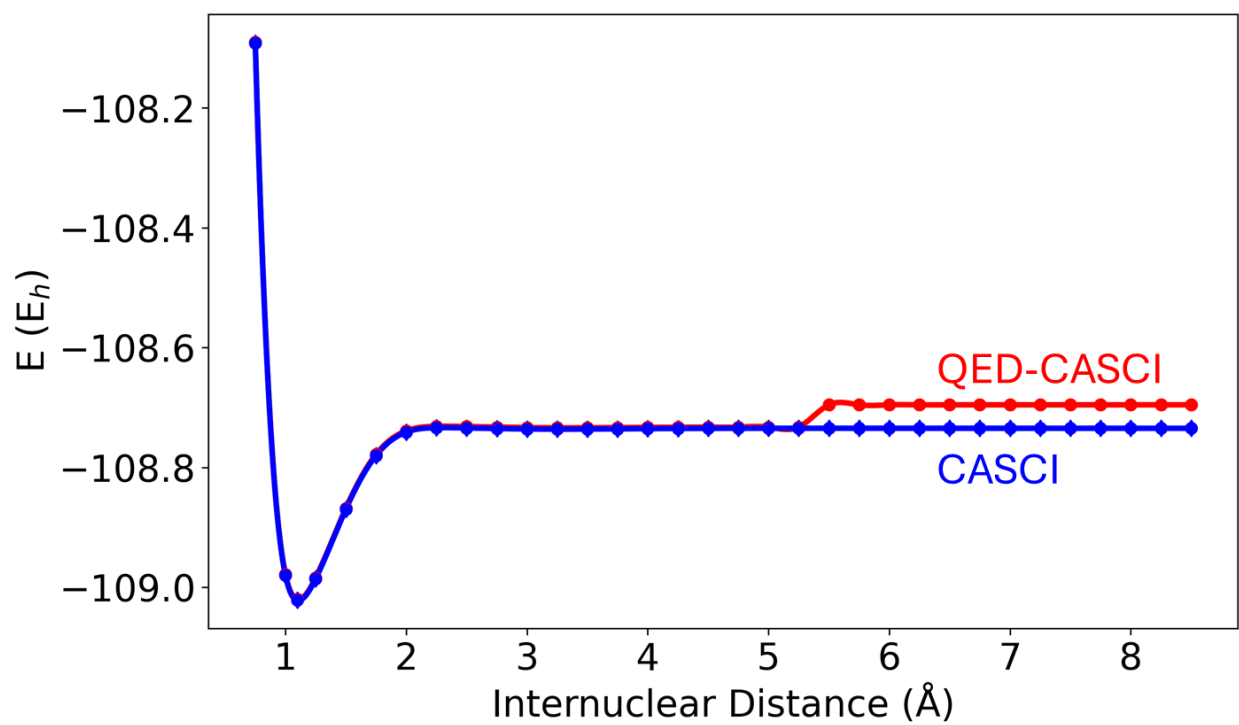

Figure S1: Comparison between the CASCI and QED-CASCI potential energy curves for the nitrogen molecule
